# Supplementary material for: Packing Confined Hard Spheres Denser with Adaptive Prism Phases
Source: arXiv:1211.6361 source file (2012-11-27)
Supplement: Supplementary file 1 [file supmat.pdf]

# Packing confined hard spheres denser with adaptive prism phases: Supplemental Material

Erdal C. Oğuz,[1,*] Matthieu Marechal,[1] Fernando Ramiro-Manzano,[2] Isabelle Rodriguez,[3,4] René Messina,[1,5] Francisco J. Meseguer,[3,4] and Hartmut Löwen[1]

[1]*Institut für Theoretische Physik II: Weiche Materie, Heinrich-Heine-Universität Düsseldorf, Universitätsstraße 1, 40225 Düsseldorf, Germany*
[2]*Nanoscience Laboratory, Dept. Physics, University of Trento, Via Sommarive 14, I-38050 Trento, Italy*
[3]*Centro de Tecnologias Fisicas, Unidad Asociada ICMM/CSIC-UPV, Universidad Politécnica de Valencia, Av. Los Naranjos s/n, 46022 Valencia, Spain*
[4]*Instituto de Ciencia de Materiales de Madrid CSIC, 28049 Madrid, Spain*
[5]*Institut de Chimie, Physique et Matériaux (ICPM), Université de Lorraine, 1 Bld Arago, 57078 Metz - Cedex 3, France*

(Dated: October 11, 2012)

## Candidate structures for the penalty method

To investigate the close-packing of hard spheres as a function of $H/\sigma$ we considered a broad set of candidates of crystalline lattices in our numerical optimizations. For confined hard spheres, the possible candidates are three-dimensional crystals with two-dimensional periodicity in the plane parallel to the confining plates. We assumed the primitive cell of these candidates to be a parallelepiped containing $k$ particles which are distributed, not necessarily evenly, on $n$ layers. For $k > 4$, we restricted ourselves to layered situations with an up-down inversion symmetry in the averaged occupancy reflecting the up-down symmetry of the confining walls. Under this sole restriction we took into account possible candidates with $k = 1, \ldots, 8$ and $n = 1, \ldots, 6$. In order to maximize the volume fraction $\phi$, we numerically optimized the cell shape and the particle coordinates. In addition, we included the unusual asymmetric buckling phases as reported in [1–3] into our candidate set, which break the up-down symmetry of the confining slit. For higher layer and particle numbers, $n \geq 6$ and $k > 8$, however, the optimization process offered difficulties due to large number of involved parameters. Hence, we fixed the particles within the prisms and we optimized their basis symmetry. Additionally, we adjusted the relative positions of the prisms and the vectors that span the unit cell for the prism phases with $k = 12$. Please also note that denser packed structures could occur with larger unit cells. However, the number of particles in each unit cell are sufficiently large to obtain all hitherto proposed structures.

## Experimental details

In our wedge cell, we used hydrophilic treated glass as substrate (3 cm large) and hydrophobic polystyrene as covering plate. We attached a 6 $\mu$m thick Mylar film along just one rim of the slides to separate the plates of the wedge cell.

We tightened the cells with several binder clips. We employed Polystyrene particles of different sizes ranging from 245 nm up to 800 nm in diameter (Ikerlat Polymers) in different experiments. We washed and rinsed the particles several times with deionized water (18.2 M$\Omega$cm). We put several drops of 1% (w/w) aqueous suspension of particles into a 2-cm-high glass tube attached to the covering plate of the cells, where the particles entered from the tube to the cells by capillarity forces through a small hole drilled on the covering plate.

The water evaporation concentrated the particles and after several days the system condensed into several facets. Finally, after the sample was dried, we detached the Polystyrene covering plate with almost no damage to the crystalline structures.

## Simulation details

The horizontal cross-section of the simulation box was allowed to deform to a general parallelogram [4], for instance, upon a crystal–crystal transition. Nevertheless, transitions between square symmetry and hexagonal symmetry phases were not observed for some values of $H$, so both square and hexagonal layers

were used as initial conditions: An fcc (100) or (111) crystal was expanded horizontally/vertically to allow an overlap-free initial condition that just fits in the slit. The number of layers $n$ was adjusted to obtain the maximum density. We performed five separate runs for each initial configuration and, if these in total 10 runs did not all result in the same final structure, we chose the maximum density configuration, which is justified by the high pressure.

## Triangular prisms

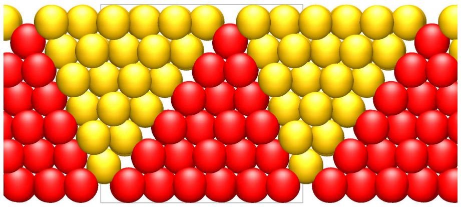

FIG. S1. The $6P_{\triangle}$ phase found for $5.73(3) \lesssim H/\sigma \lesssim 5.88(3)$ from Monte Carlo simulations. (The snapshot is periodically repeated; the original simulation box is indicated by the gray rectangle.)

## Degeneracy in the rhombic phases

Recent simulation work [5] and theoretical [6, 7] investigations show that the buckling phase $2B$ as well as the bilayered rhombic phase $2R$ are highly degenerated as there exists linear and zig-zag ordering of the unit cells in the corresponding phase structures. Likewise, we studied the phase behavior of rhombic phases $nR$ for $n = 3, 4$ closer. As a result, we notice that higher layered rhombic phases are degenerated in the same way: we found zig-zag rhombic in addition to the linear one. The corresponding structures are illustrated in Fig. S2.

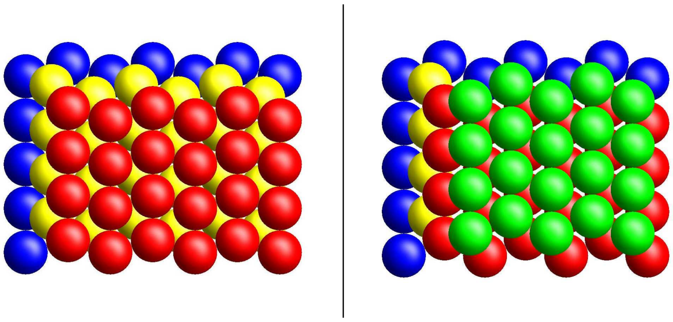

FIG. S2. Zig-zag orderings in the phase structures $3R$ (left) and $4R$ (right). In addition to linear ordering of the unit cells of these phases, we also found close-packed zig-zag ordering yielding a degeneracy in the packing fraction. Different colors correspond to different layers parallel to confining walls.

* ecoguz@thphy.uni-duesseldorf.de; http://www2.thphy.uni-duesseldorf.de/~ecoguz/


[1] T. Chou and D. R. Nelson, Phys. Rev. E **48**, 4611 (1993).
[2] H. Löwen, Soft Matter **7**, 8050 (2010).
[3] H. Bock, K. E. Gubbins, and K. G. Ayappa, J. Chem. Phys. **122**, 094709 (2005).
[4] R. Najafabadi and S. Yip, Scripta Metall. **17**, 1199 (1983).
[5] A. Fortini and M. Dijkstra, J. Phys.: Condens. Matter **18**, 371 (2006).
[6] M. Schmidt and H. Löwen, Phys. Rev. Lett. **76**, 4552 (1996).
[7] M. Schmidt and H. Löwen, Phys. Rev. E **55**, 7228 (1997).
